# Supplementary material for: Deep Data Flow Analysis
Source: arXiv:2012.01470 source file (2020-11-21)
Supplement: Supplementary file 1 [file supplementary_material.tex]

\title{Deep Data Flow: Appendices}

\maketitle

\appendix
\input{appendix/dataflow_problems}
\input{appendix/dataset}
\input{appendix/experimental_setup}
\input{appendix/downstream_tasks}

\bibliography{refs}
\bibliographystyle{iclr2021_conference}
